# Supplementary material for: Bidirectional Autoregressive Diffusion Model for Dance Generation
Source: arXiv:2402.04356 source file (2024-06-22)
Supplement: Supplementary file 1 [file X_suppl.tex]

\clearpage
\setcounter{page}{1}
\maketitlesupplementary

\paragraph{FID results.}
As claimed in EDGE, the FID metrics present limitations since AIST++ test set does not thoroughly cover the train distribution.
Even so, we also present the FID results in Table~\ref{r1}. We use the codes from Bailando. The FACT and Bailando results were reported from their original papers.  Our method gets the best results except for the $\text{FID}_\text{g}$ of Bailando, demonstrating its capability to generate smoother sequences. Bailando focuses on organizing the movements, and $\text{FID}_\text{g}$ metric reflects the quality of
choreography.

\begin{table}[h]
\centering

\footnotesize
 \resizebox{0.25\textwidth}{!}{
\begin{tabular}{l|cc}
\toprule
	  
Method &  $\text{FID}_\text{k} \downarrow$ & $\text{FID}_\text{g} \downarrow$   \\
\midrule
GT  &17.10 & 10.60\\
\midrule
FACT   & 35.31& 22.11 \\
Bailando   & 28.16& \textbf{9.62} \\
EDGE   & 31.23& 24.71 \\
\midrule
Ours   & \textbf{27.02}& 20.24 \\
\bottomrule
\end{tabular}}

 \caption{FID results of the different methods.}
\label{r1}
\vspace{-10pt}
\end{table}

\paragraph{The reason for using $z_{k+1}$ in AR encoder.}
According to the characteristics of the DDPM diffusion model, as the timestep t increases, the added noise becomes increasingly subtle. Consequently, the noised sequence bears a greater resemblance to the original one. 
$z_{k+1}$  progressively offers clearer insights about the future sequence.
Also, from the FID results in Table~\ref{r2}, it can be seen that the model using a bidirectional encoder yields smoother results compared to the model using a unidirectional encoder.

\begin{table}[h]
\centering

\footnotesize
 \resizebox{0.25\textwidth}{!}{
\begin{tabular}{l|cc}
\toprule
	  
Method &  $\text{FID}_\text{k} \downarrow$ & $\text{FID}_\text{g} \downarrow$   \\
        \midrule
       EDGE   & 31.23& 24.71 \\
        \midrule
           w/o Beat    & 27.60& 20.94 \\
           Unidirection  & 28.24& 22.28 \\
            w/o LID    &28.31 &22.51 \\
           \midrule
           Ours   & \textbf{27.02}& \textbf{20.24} \\
        \bottomrule

\end{tabular}}

 \caption{FID results of the different settings.}
\label{r2}
\vspace{-10pt}
\end{table}

\paragraph{Details about diffusion process.} 
We employ DDPM to elaborate on the entire diffusion process, with a diffusion timestep set to 1000. Throughout the training, we randomly select the time step t in each iteration, effectively constraining the training time. 
For inference, we leverage DDIM for expediting sampling.

\paragraph{Inference spreed.}
In our setting, EDGE requires 9.54 seconds to generate a 5-second dance sequence, while our method takes 10.45 seconds. Although our method incurs a slightly higher time cost, the difference is marginal.
